# Supplementary material for: Quantum modulation of a coherent state wavepacket with a single electron spin
Source: arXiv:2207.05596 source file (2022-07-12)
Supplement: Supplementary file 1 [file Supplement_experiment.pdf]

# Supplementary Information

## I. SAMPLE INFORMATION

The system under consideration is a micropillar photonic structure. The sample has been fabricated via molecular beam epitaxy (MBE) and contains a $\lambda$-thick cavity surrounded by two distributed Bragg reflectors (DBRs). The DBR structure consists of 18.5 (5) bottom (top) AlAs/GaAs mirror pairs. A modulation doped low density In(Ga)As QD layer ($\sim 1.8 \times 10^9 cm^{-2}$) has been grown in the middle of the cavity. The QDs have been grown spectrally close to the cavity mode resonance at $\sim 893nm$, with a Q-factor $\sim$ 300 in a $2\mu$m diameter etched micropillar. The low Q-factor micropillar cavity can increase the light-matter interaction such that we are able to observe a bright RSF signal from the QD even in the weak drive regime. Of greater significance is that the low Q-factor ensures we can neglect any cavity induced birefringence as the bandwidth of the cavity mode is orders of magnitude larger than any polarisation mode splitting resulting from asymmetry in the shape of the cylindrical pillar.

## II. NEUTRAL QD

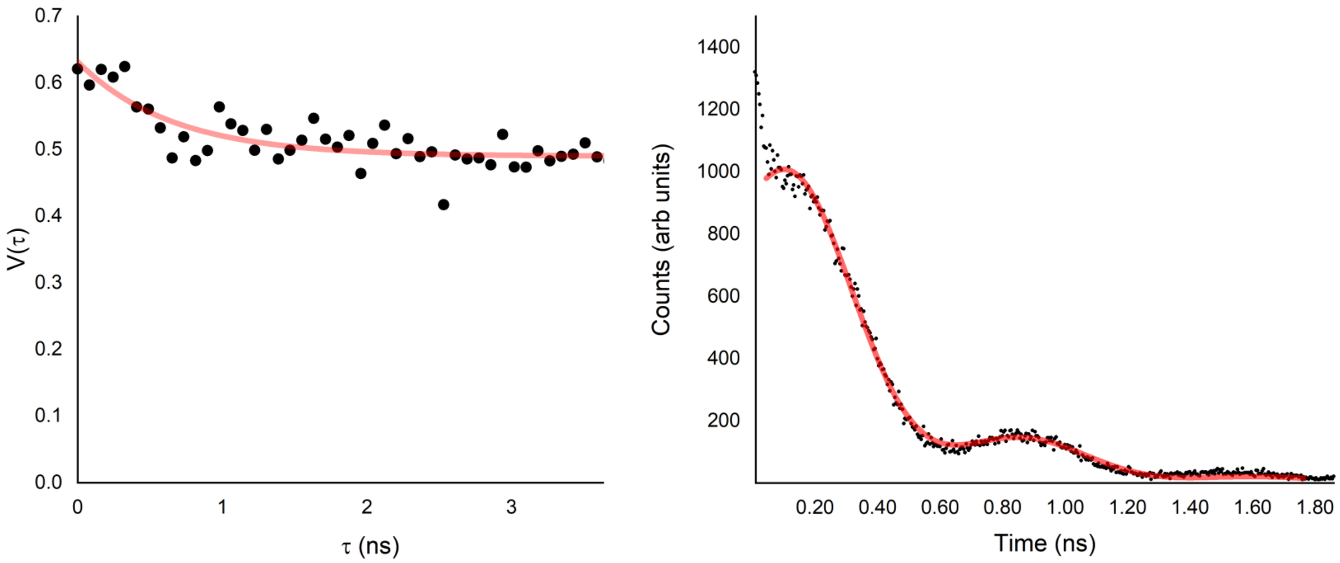


FIG. 1: Left is the visibility of the interference measured using the setup in Fig.1.(a) from the main paper for a neatral QD. Right lifetime for the QD from measured under Pulsed RF conditions. Both data sets are recorded at a $B \sim$ 100mT Voigt field

We also perform a reference measurement on a neutral QD so the $|g^{(1)}|$ can be compared to the results in the main paper this can be seen in Fig.1. Here we see a small initial decay in the coherence as a result of real excitation which then levels out to give a flat $V(\tau)$ corresponding to the RSF field inheriting the coherence of the laser [1]. We also measure the lifetime as we did for the charged QD. Interestingly the decay from real excitation now contains oscillations these are a beating between the two possible excited state transitions. This is possible as they share a common ground state unlike the charged QD of the main paper. The oscillations correspond to a line splitting $\sim 0.9\mu$eV, likely due to fine structure splitting that the $B \sim$ 100mT Voigt field applied here is unlikely to have overcome. The observed decay time corresponds to a fourier transform limited linewidth $\sim 1.6\mu$eV, hence this QD exhibits a sub natural linewidth splitting. The amplitude modulation that is observed for the neutral QD here is in contrast with the charged QD that contains a ground state spin, where there is no beating in the optical lifetime ($0.3\mu$eV Zeeman splitting). This is due to the fact that output photons become entangled with the ground state spin preventing interference. This leaves a modulation that is purely on the phase of the RSF field.

## III. MASTER EQUATION MODEL OF DRIVEN QD SPIN

The system under consideration in this work can be modeled as a four level system (FLS), spanned by the states $\{|\Uparrow\rangle, |\uparrow\rangle, |\downarrow\rangle, |\Downarrow\rangle\}$, coupled to two cavity modes, $a_L$ and $a_R$, representing left and right circular polarisation respectively. These cavity modes are then coupled to port modes $r_{k,L}$ and $r_{k,R}$ where again $L$ and $R$ denote left and right circular polarisation. With this we can express the Hamiltonian of the full system as $H = H_0 + H_B + H_I$. Where $H_0$ represents the energy of the FLS and cavity, $H_B$ represents the energy of the port modes and $H_I$ describes the interactions between the subsystems. Furthermore these can be expressed in terms of the system parameters as follows

$$H_0 = \omega_0 P_e + \omega_B \sigma_x + \omega_c(a_R^\dagger a_R + a_L^\dagger a_L) \tag{1}$$

$$H_B = \sum_k \omega_k (r_{k,R}^\dagger r_{k,R} + r_{k,L}^\dagger r_{k,L}) \tag{2}$$

$$H_I = g(S_-^R a_R^\dagger + S_-^L a_L^\dagger + \text{H.c.}) + \sum_k \kappa_k (r_{k,R} a_R^\dagger + r_{k,L} a_L^\dagger) + \text{H.c.}. \tag{3}$$

Here, $P_e = |\Uparrow\rangle\langle\Uparrow| + |\Downarrow\rangle\langle\Downarrow|$ is the projection operator on to the excited state subspace, $\omega_B\sigma_x = \omega_B(|\uparrow\rangle\langle\downarrow| + |\downarrow\rangle\langle\uparrow|)$ represents the coupling of the ground states caused by the external magnetic field in the Voigt geometry, $S_-^R = |\uparrow\rangle\langle\Uparrow|$, $S_-^L = |\downarrow\rangle\langle\Downarrow|$ and finally $g$ and $\kappa_k$ represent coupling constants. To calculate the quantities we are interested in requires a master equation for the dynamics of the FLS. To arrive at this we follow methods described in [2]. Hence, the port modes are traced out giving a master equation for the cavity and the FLS in the Born Markov approximation. Furthermore, the cavity modes can be eliminated adiabatically [3] leading to the following master equation written in a frame rotating at the drive field frequency

$$\dot{\rho}(t) = -i[H, \rho(t)] + \sum_{k=R,L} L_k \rho(t) L_k^\dagger - \frac{1}{2}\{L_k^\dagger L_k, \rho(t)\} + \mathcal{D}(\rho), \tag{4}$$

with

$$H = \Delta P_e + \omega_B \sigma_X + (\Omega_R S_-^R + \Omega_L S_-^L + H.c.). \tag{5}$$

The Lindblad operators responsible for optically induced dissipation have the form $L_{R/L} = \sqrt{\Gamma} S_-^{R/L}$ and $\mathcal{D}(\rho) = \sigma_x \rho(t) \sigma_x - \frac{1}{2}\{\sigma_x^2, \rho(t)\}$ describes the additional process of pure-dephasing. Here $\Delta$ is the renormalised detuning, $\Gamma$ is the Purcell enhanced decay rate and $\Omega_{R/L}$ represents the driving parameters of the system. This adiabatic approximation is valid in the regime where the cavity bandwidth is much greater then the bandwidth of the system dynamics.

We define the visibility, $V(\tau)$, of the RSF as measured by the MZI as the magnitude of the steady state first order correlation function and the cross polarised emission spectrum $S(\omega - \omega_D)$ as the Fourier transform of this same correlation function. Mathematically this gives us

$$V(\tau) = \left| g^{(1)}(\tau) \right| \tag{6}$$

$$S(\omega - \omega_D) = \int_{-\infty}^{\infty} g^{(1)}(\tau) e^{-i\omega\tau} d\tau \tag{7}$$

To calculate this steady state correlation function we express it in terms of the vertically polarised output electric field.

$$g^{(1)}(\tau) = \langle \mathbf{E}_V^{(-)}(\tau) \mathbf{E}_V^{(+)}(0) \rangle \propto \langle S_+^V(\tau) S_-^V(0) \rangle, \tag{8}$$

Where the final proportionality can be derived by applying input-output theory [4] to the system and holds when the input field is horizontally polarised. With the desired quantities now expressed in terms of operators of the FLS they can be calculated by solving the master equation numerically. Here this was done via QuTiP [5] which we use to generate the plots in Fig.2 in the main paper. A more detailed derivation and treatment of the master equation can be found in [6].

## IV. SPECTRAL JITTER AND DEPHASING

In Fig.2 in the main paper we use the master equation model from the previous section to predict how the RSF spectrum varies with QD-laser detuning. Fig.2.(a) shows the inhomogeneously broadened spectra of QD1 described in Fig.1 and Fig.2 in

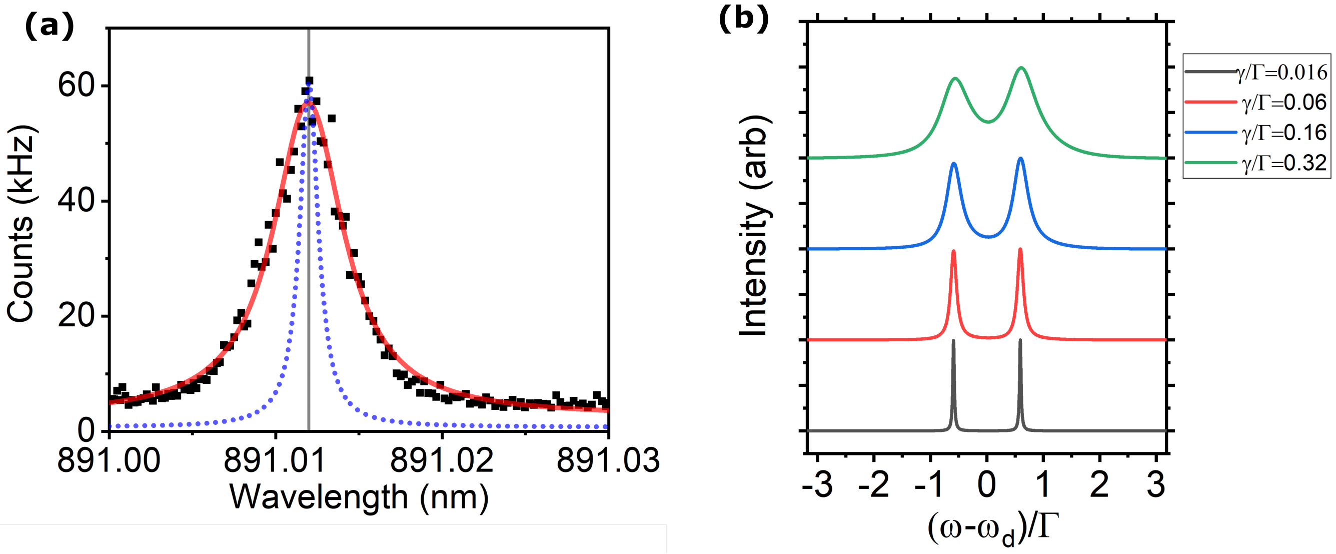


FIG. 2: (a) Shows a The RSF spectrum as a function of the drive field laser wavelength. Data is recorded by stepping the wavelength single frequency laser and integrating the number of counts in the V-polarised channel over a 1 second interval at each wavelength. The blue dashed line is an indicator that represents the transform limited result derived from the observed spontaneous emission lifetime. The grey solid line represents the drive field laser spectrum for the case when $\Delta = 0$. (b) Shows the affect of varying the pure dephasing rate in the master equation has on the RSF spectrum for the case when the QD-laser detuning is set to $\Delta/\Gamma = 0.5$. It is clear as the pure dephasing rate is decreased the asymmetry in the RSF disappears.

the main paper. The data is accumulated by tuning the single frequency drive laser through the QD transition where we observe a RSF signal with a Lorentzian line-shape and bandwidth of $\sim 5\mu$eV. This is substantially broader than the $\sim 1.3\mu$eV of the transform limited line and shows the extent to which spectral jitter broadens the observed transitions. Over the course of an experimental run ($>$ seconds) if our single frequency laser remains at a fixed frequency then the QD will be subjected to this slow ($\sim \mu$s) spectral jitter and the Fourier limited line will (randomly) explore a full range of detunings. We showed that the output RSF is invariant to this detuning and thus remains unchanged in all aspects besides it's intensity.

At moderate values for the QD-laser detuning ($\Delta/\Gamma = \pm 0.5$) there is an observable discrepancy between the peak heights in the RSF spectrum. This is an artefact of the the way dephasing is modelled in the master equation. In order to ensure the master equation can describe the experiment we need to incorporate a term that describes spin dephasing. The established way to do this is by adding a Linblad term $\mathcal{D}(\rho)$. This models a pure dephasing process ($\gamma$) which is the equivalent to the $T_2$ coherence time for the spin. Whilst the RSF from the QD-spin is invariant to spectral wander that stark shifts the transitions it is not insensitive to changes in the Larmor frequency (Zeeman splitting). These processes fall more broadly under the umbrella of spin noise. Here slow (of order $\mu$s) variations to the nuclear spin bath cause a time varying Overhauser field across the QD. This dynamically changes the effective B-field applied to the QD-spin and changes the Line splitting in the RSF. When this is averaged over longer timescales ($>$ seconds) it leads to an inhomogeneous broadening where experimentally one measures the $T_2^*$. Since our measurements cannot distinguish the $T_2$ from the $T_2^*$ we use a model with pure dephasing i.e. $T_2$. This represents a worse case scenario for the dephasing of the spin as the underlying $T_2$ in our system is likely significantly longer and we are dominated by inhomogeneous processes.

The pure dephasing model is responsible for the discrepancies in peak heights in the RSF. We can see from Fig.2.(b) as the rate of pure dephasing approaches the that of the spontaneous emission lifetime the asymmetry in the RSF spectrum is more pronounced. This is due to the addition of a competing incoherent process that becomes sensitive to the small Zeeman splitting at moderate detunings. Clearly in the limit where the pure dephasing is small this effect is not observed and the underlying RSF spectrum is derived from coherent processes and the spectrum retains its symmetry. By using a model of pure dephasing we over emphasise this effect where in the limit of no pure dephasing and the observed coherence is entirely limited by inhomogeneous effects then the spectrum would be symmetric for all values of $\Delta$. A more detailed study of the dephasing mechanisms can be found in [6]

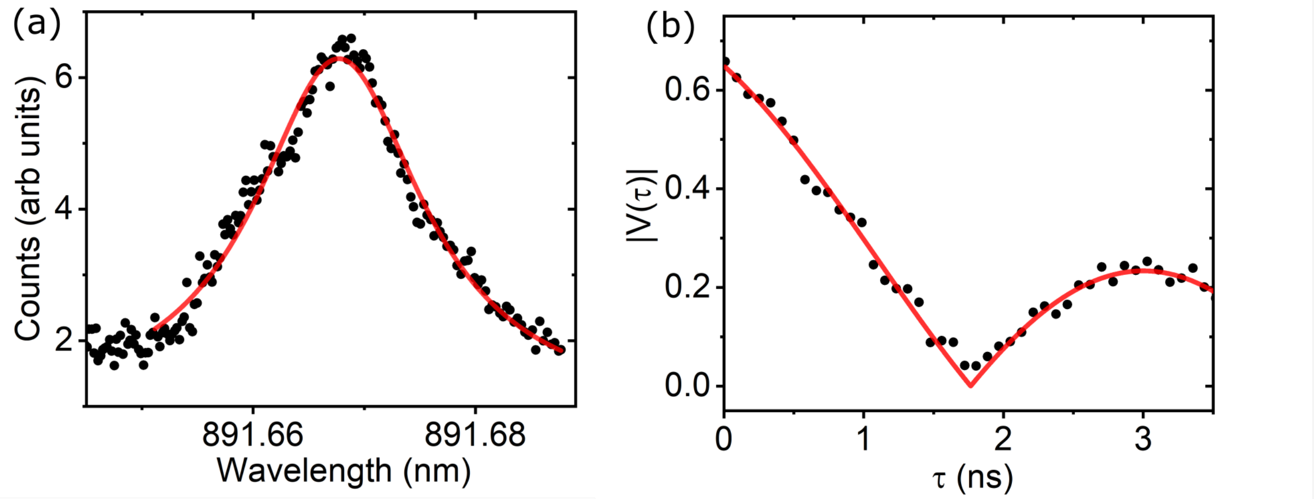


FIG. 3: (a) The RSF response as a single frequency laser is tuned through the QD2 transition for a drive strength $\omega \sim 0.1\Gamma$ in a $B \sim$ 86mT Voigt field. The measured linewidth is $\sim 28\mu$eV this is considerably broader than QD1 due to an increase in the spectral jitter for this particular QD (b) Measurement of $|g^{(1)}(\tau)|$ for QD2 under the same driving conditions. Fitting the data yields a time period for the precession $\sim$ 6.2ns or a Larmor precession frequency $2\omega_B \sim$ 157MHz i.e a Zeeman splitting $\sim 0.1\mu$eV. This matches the timescales recorded for the homodyne measurement in the main paper.

## V. SUPPLEMENTARY DATA FOR QD2

For stabilised homodyne measurements we use QD2 this is due to its lower in plane gyromagnetic ratio. In Fig3.(b) we can see the $|g^{(1)}(\tau)|$ which corresponds to a Larmor precession frequency of $2\omega_B \sim$ 157MHz for $B \sim$ 86mT. This is approximately three times slower than QD1 which means the two photon correlations from the homodyne interferometer can be captured with standard Si-APDs with around 30% efficient detection with a timing uncertainty $\sim$ 300ps. Statistics for the each homodyne measurement are gathered over approximately 24 hours. Note we do not use the same thin film APDs that are deployed to measure QD1 as the efficiency is only a few % which for this particular measurement makes two photon correlations challenging.

The disadvantage of QD2 is that the slow precession frequency means the $|g^{(1)}(\tau)|$ is less reliable. In order for the fitted data to be reliable we need to observe at least one full oscillation the data in Fig3.(b) only contains a half period. This is why in the main paper we focus on QD1 for a discussion of the dynamics observed in the $|g^{(1)}(\tau)|$, and also why the values quoted above are only given approximately.

[1] S. Ates, S. M. Ulrich, S. Reitzenstein, A. Löffler, A. Forchel, and P. Michler, Phys. Rev. Lett. **103**, 167402 (2009), `https://link.aps.org/doi/10.1103/PhysRevLett.103.167402`.
[2] H. Carmichael, *Statistical Methods in Quantum Optics 1* (Springer, Berlin, 2002).
[3] H. J. Carmichael, *Statistical Methods in Quantum Optics 2* (Springer-Verlag, 2008).
[4] C. W. Gardiner and M. J. Collett, Phys. Rev. A **31**, 3761 (1985).
[5] J. Johansson, P. Nation, and F. Nori, Computer Physics Communications **184**, 1234 (2013), ISSN 0010-4655, `https://www.sciencedirect.com/science/article/pii/S0010465512003955`.
[6] T. N. et al, Manuscript in preparation (2022).
